# Supplementary material for: Looking 3D: Anomaly Detection with 2D-3D Alignment
Source: arXiv:2406.19393 source file (2024-06-27)
Supplement: Supplementary file 1 [file X_suppl.tex]

\clearpage
\setcounter{page}{1}
\maketitlesupplementary

% HB: Things to add
% \begin{itemize}
%     \item 3DPE: dimension of Fourier encoding, details
%     \item Training details of baselines LFD, Lin et al
%     \item Training details of our model, e.g. which loss function is used to update which parameters
%     \item Details of viewpoint estimation, it is a classification problem, how gt is chosen, baseline details, how many bins for viewpoint, number of epochs, etc
%     \item How do we sample positive/negative for VLFA?
%     \item Examples for anomaly localisation
%     \item Any missing details about real data experiments?
%     \item User study: Show examples where humans fail, do better and worse than ours
% \end{itemize}

In this supplementary material, we present additional details of the dataset creation pipeline, implementation details, and qualitative results. In Sec.~\ref{sec:dataset}, we provide additional details of our proposed dataset, Sec.~\ref{sec:impl} presents additional implementation details of the CMT and other baselines. Sec.~\ref{sec:bbox} illustrates the qualitative results of the anomaly localization task. Sec.~\ref{sec:view} provides additional information and qualitative results of the view prediction experiment and Sec.~\ref{sec:unseen} shows experiments on unseen categories. Finally, Sec.~\ref{sec:user} presents additional details of the user study experiments. 

\section{Additional Details of \dname}
\label{sec:dataset}
\noindent \textbf{Deformation parameters.} We normalize the vertices to $[-1,1]$ before applying geometric deformation. For positional anomaly, we randomly translate the vertices of a random part by an offset of $\delta p$. The translation offset for each axis is randomly sampled from a uniform distribution of range $0.04\leq |\delta p| \leq 0.08$. To create rotational Anomalies, we apply a 3D rotational transformation to a random part. The rotation matrix is formed using a random rotation axis and an angle ($r_\theta$, radians) sampled from a uniform distribution of range $0.2\leq |r_\theta| \leq 0.4$. The center of rotation is set to a fixed point at one of the connecting points between the anomalous part and the main body of the chair object. 

\noindent \textbf{Quality control and verification.} 
We aim to ensure that the resulting anomaly shapes adhere to the principles of physics. For instance, in case of positional and rotational anomaly, if a part detaches from the chair's main body during the deformation process such that it stands itself, we reject the generated anomaly and initiate the process again, adjusting the parameters as necessary. \textcolor{black}{Similarly, for missing anomaly types, if removing a specific part makes the chair structurally impractical, we discard the sample and attempt to remove a different part of the same chair instance.} %Similarly, for missing part anomaly types, we do not remove any part that can make the chair structurally impractical. 
% \CJ{not clear. Does this mean you do not remove a whole part?} 
For broken anomaly types, if a particular break removes more than 90\% or less than 10\% of an object we discard the sample and regenerate another break. %After 5 attempts, we discard the specific part and try with a different part. 

We also apply an IoU thresholding technique (see Fig.~\ref{fig:view}) to filter out rendered samples in cases where the created anomaly closely resembles its normal counterpart primarily because of the camera viewpoint. To do this, we generate masks for the working part both before and after applying the deformation. Subsequently, we calculate the IoU between these two masks, and if the IoU exceeds 0.8, we discard the rendered image and try with a different camera angle. If the same occurs four times in a row, we will discard that particular anomaly shape.

\noindent \textbf{Additional dataset statistics.}  Our dataset has 103 distinct part categories involving some type of anomaly. The distribution of these parts over different anomaly types is illustrated in Fig.~\ref{fig:partstats}. For the visualization, certain part categories have been grouped and are shown in the Figure. Fig.~\ref{fig:genstats}(a) shows statistics of anomaly sizes as indicated by their normalized bounding box areas. An anomalous part can be partially occluded or hidden by other parts of the object when captured from a specific camera viewpoint. Fig.~\ref{fig:genstats}(b) illustrates the degree of occlusion within our dataset. Rendered instances where anomalies are entirely occluded are excluded from our dataset.

\begin{figure}[t!]
\begin{center}
   \includegraphics[width=0.9\linewidth]{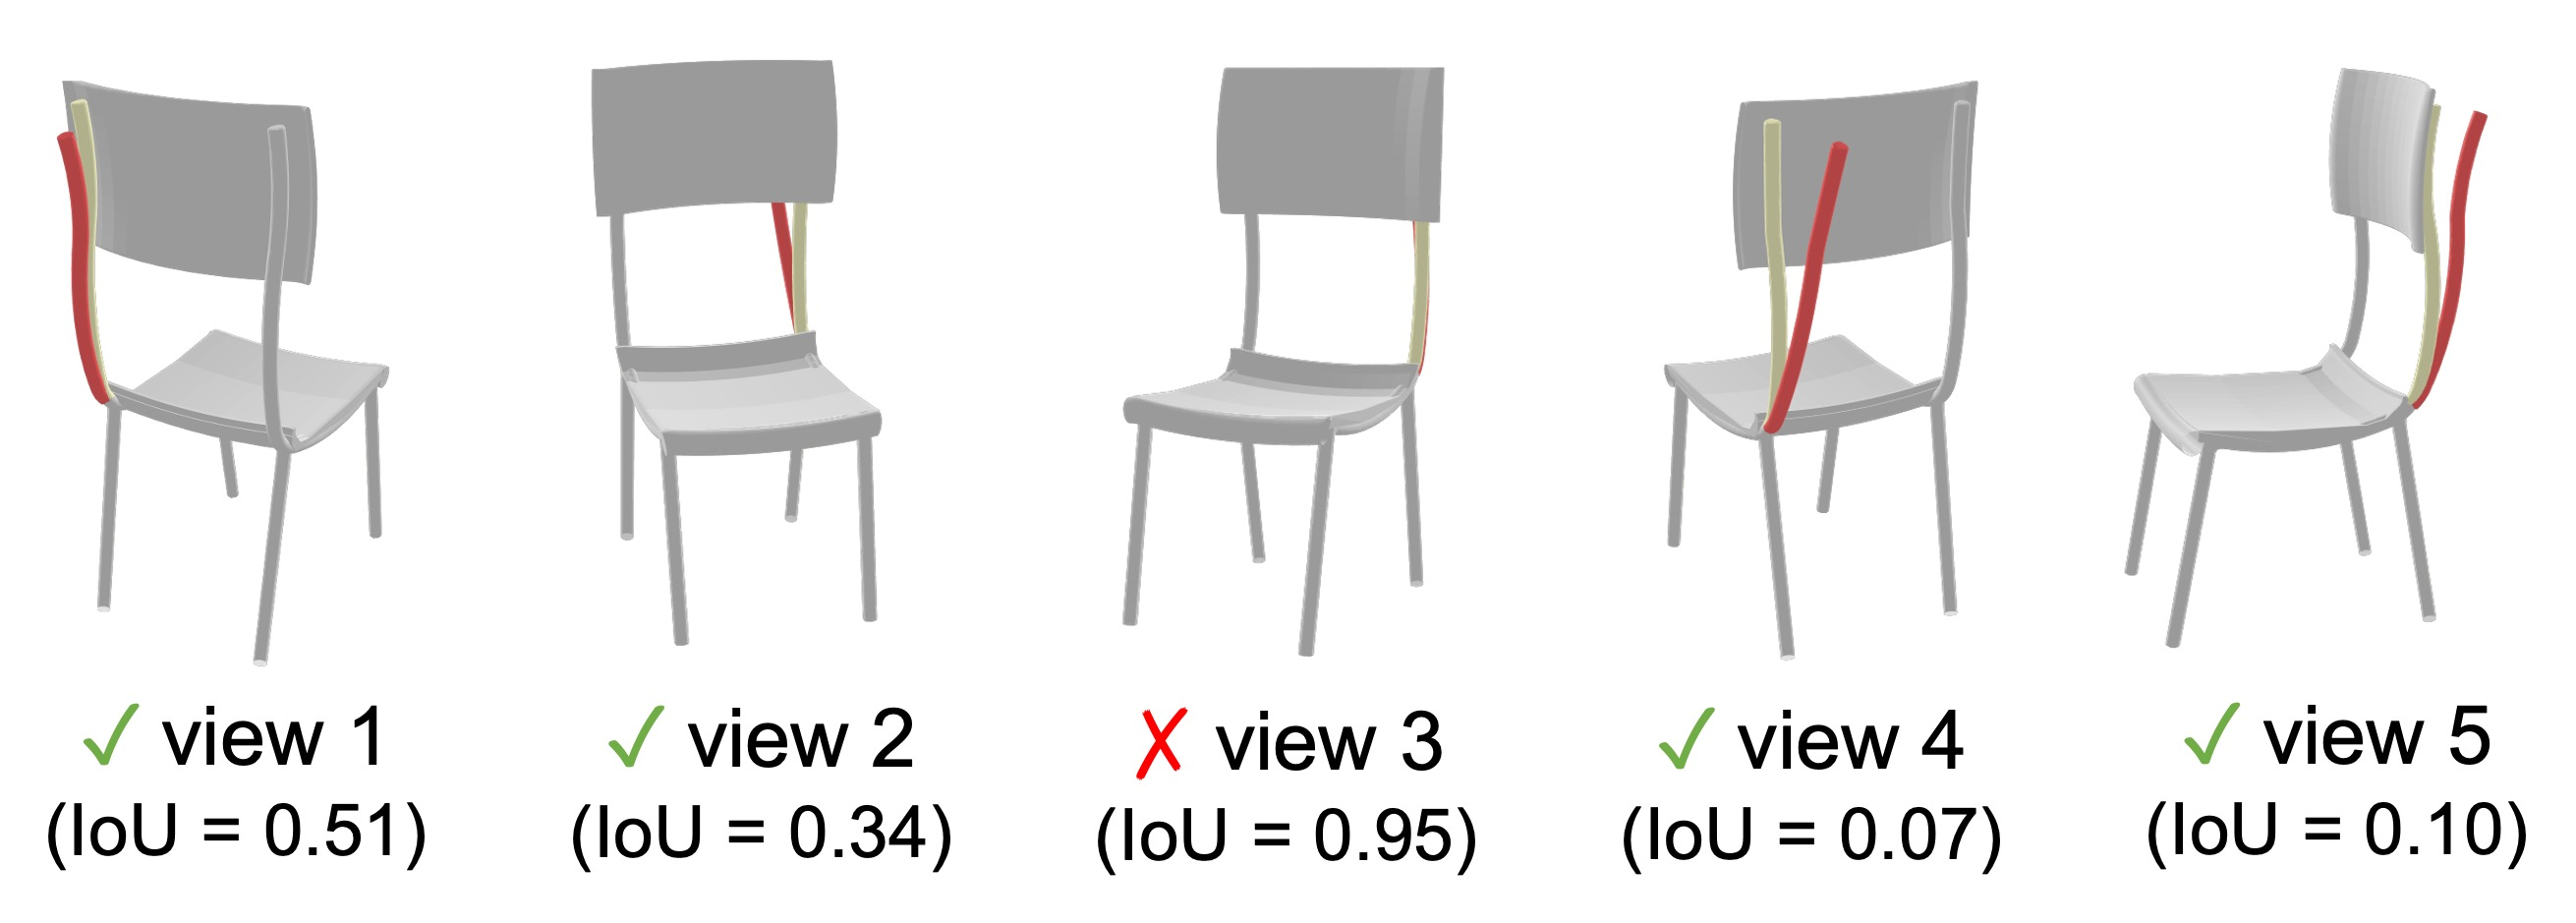}\vspace{-0.5cm}
\end{center}\vspace{-0.2cm}
\caption{IoU-based thresholding to filter out rendered samples where the created anomaly (red) closely resembles its normal counterpart (yellow). We generate masks before and after deformation, calculate their IoU, and if it's over 0.8, we discard the rendered sample.}

\label{fig:view}
 \vspace{-0.3cm}
\end{figure}

\begin{figure}[t!]
\begin{center}
   \includegraphics[width=1\linewidth]{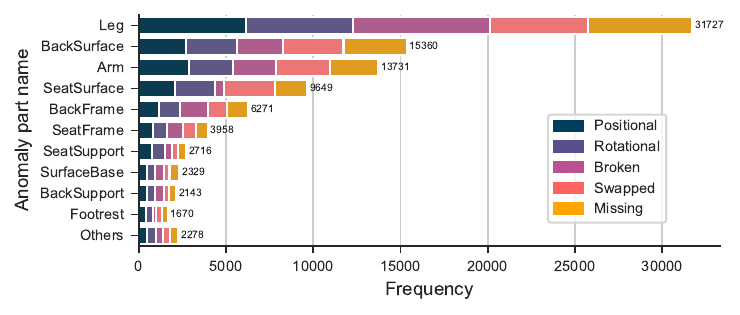}\vspace{-0.5cm}
\end{center}\vspace{-0.2cm}
\caption{Distribution of anomaly types within our dataset, categorized by salient chair parts. Each row in the plot represents the number of instances, various anomaly types are observed within the part in the whole dataset.}
\label{fig:partstats}
 \vspace{-0.3cm}
\end{figure}

\begin{figure}[t!]
\begin{center}
   \includegraphics[width=1\linewidth]{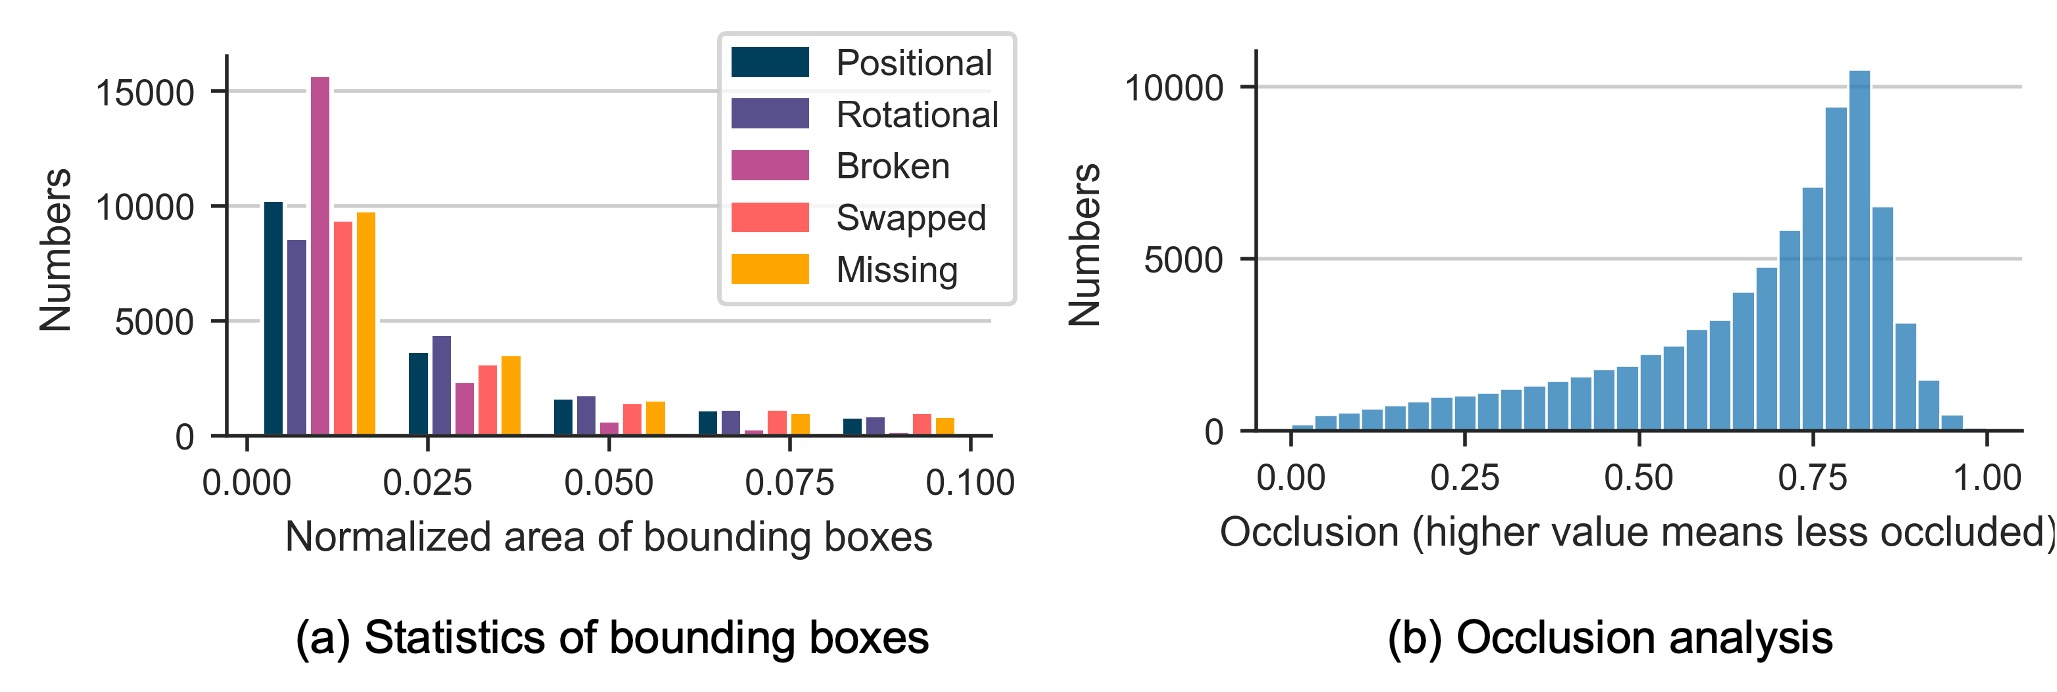}\vspace{-0.5cm}
\end{center}\vspace{-0.2cm}
\caption{\textbf{(a)} Distribution of anomaly sizes as indicated by their bounding box areas. \textbf{(b)} The histogram plot illustrates the distribution of occlusion within our dataset.  The $x$-axis of the plot denotes the fraction of the anomalous part visible. }
\label{fig:genstats}
 \vspace{-0.3cm}
\end{figure}

\begin{figure}[t!]
\begin{center}
   \includegraphics[width=1\linewidth]{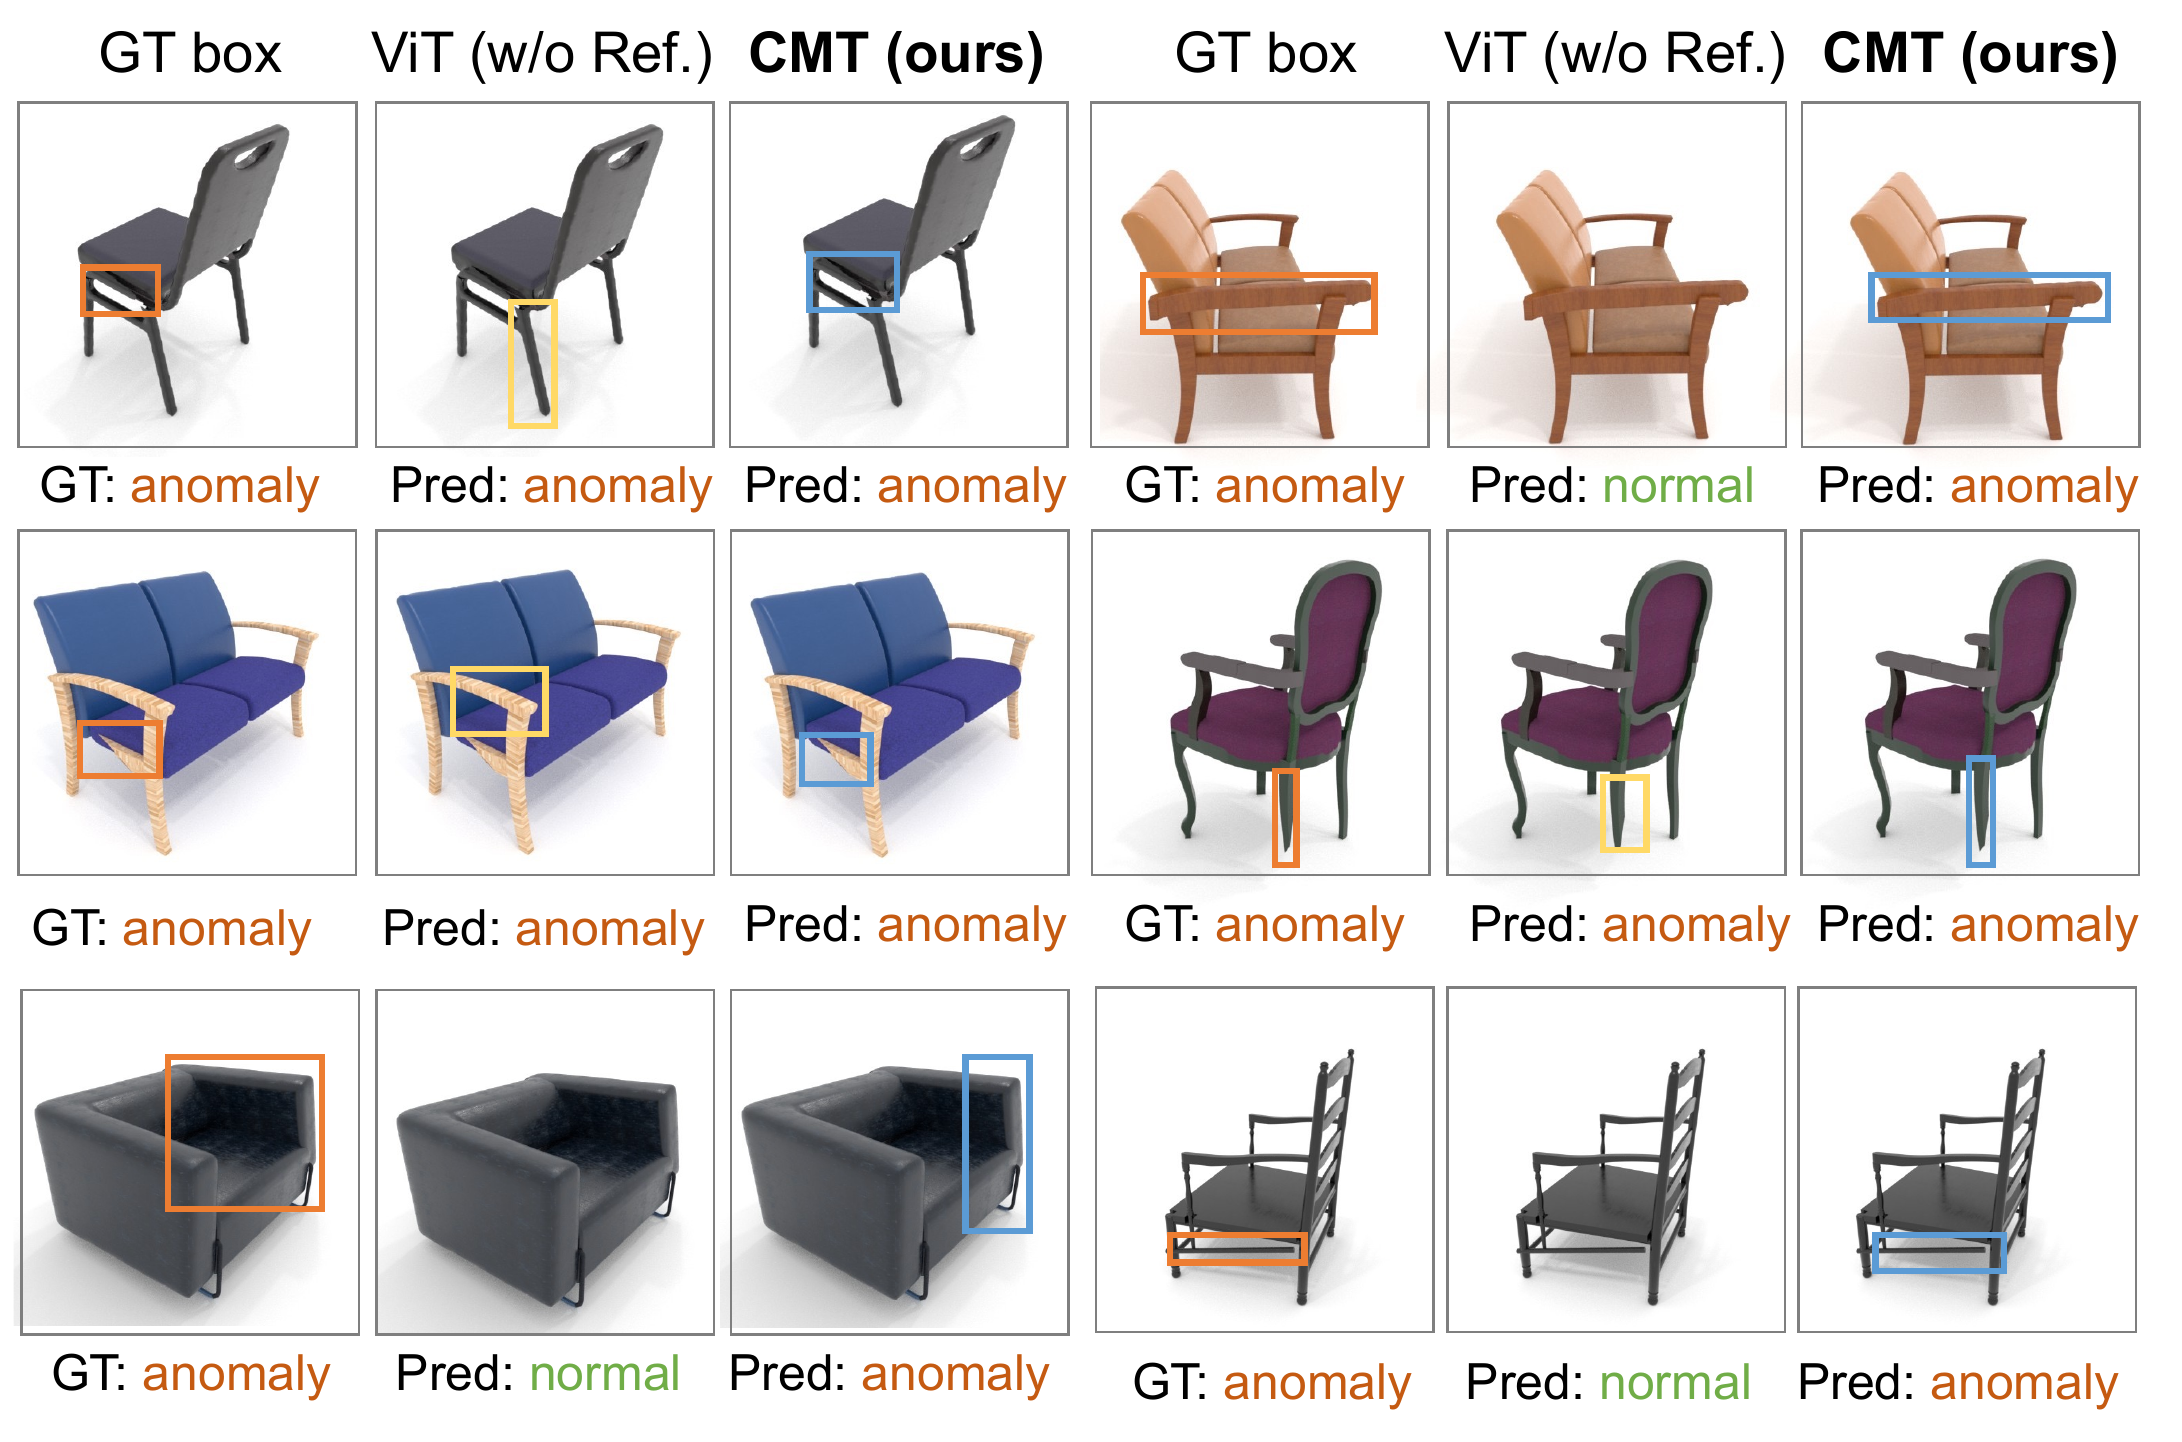}\vspace{-0.4cm}
\end{center}\vspace{-0.2cm}
\caption{Bounding box regression results. We compare our proposed CMT with ViT which does not use the 3D reference. 
}
\label{fig:bbox}
 \vspace{-0.1cm}
\end{figure}

\section{Additional Implementation Details}
\label{sec:impl}

\noindent \textbf{Architecture details of 3DPE.} We use a Fourier encoding function, denoted as $\gamma_F$, which maps $\mathbb{R}$ into a higher dimensional space $\mathbb{R}^{2l}$. Formally, the encoding is denoted as:
\begin{equation}
\begin{split}
     \gamma_F(x) = ( \text{sin}(2^0\pi x), \text{cos}(2^0\pi x) ,..., \\
     \text{sin}(2^{l-1}\pi x), \text{cos}(2^{l-1}\pi x))
\end{split}
\end{equation}
This function $\gamma_F(\cdot)$ is applied separately to each of the three coordinate values in $\bx$. After including the original coordinate values, we obtain a $6l+3$ dimensional vector. We set $l=10$ in our experiments. The output is further processed through an MLP block of $2$ linear projection layers, obtaining a final $d$ dimensional 3DPE. 

\noindent \textbf{Negative sampling in VLFA.} The view-agnostic alignment loss is calculated over a subset of $32$ feature points. For each feature point, the negatives are sampled both from non-corresponding points in the reference view of the same object and from other objects in the batch. 

\noindent \textbf{Training details of CMT.} We train our model end-to-end using the binary cross-entropy loss, denoted as $\mathcal{L}_\textup{bce}$, along with the view-agnostic alignment loss, denoted as $\mathcal{L}_\textup{va}$.
Specifically, the $\mathcal{L}_\textup{va}$ updates the parameters of $\varphi$, $\beta$. On the other hand, the $\mathcal{L}_\textup{bce}$ is used to update $\varphi$, $\gamma$, and $\phi$. Note that $\beta$ is only updated based on the alignment loss. This ensures that the view-agnostic space obtained through  $\beta$ is not affected by the classification objective.

\noindent \textbf{Training details of related works.} While the works of Grabner~\etal~\cite{grabner2019location} and Lin~\etal~\cite{lin2021single} are originally based on retrieval task, we adopt them for the conditional AD problem. Both methods follow a metric learning training scheme. In our formulation, a reference shape and a normal image form a positive pair, while an anomaly image forms a negative pair. We train the model using the loss functions described in the paper, aiming to increase the distance between the negative pair and subsequently decrease the distance between the positive pair. During inference, we calculate an L1 distance between the shape and query representation. We set a threshold value of 0.8 for both methods. If the distance is greater than the threshold we classify the query as an anomaly otherwise a normal. 

\begin{figure}[t!]
\begin{center}
   \includegraphics[width=0.99\linewidth]{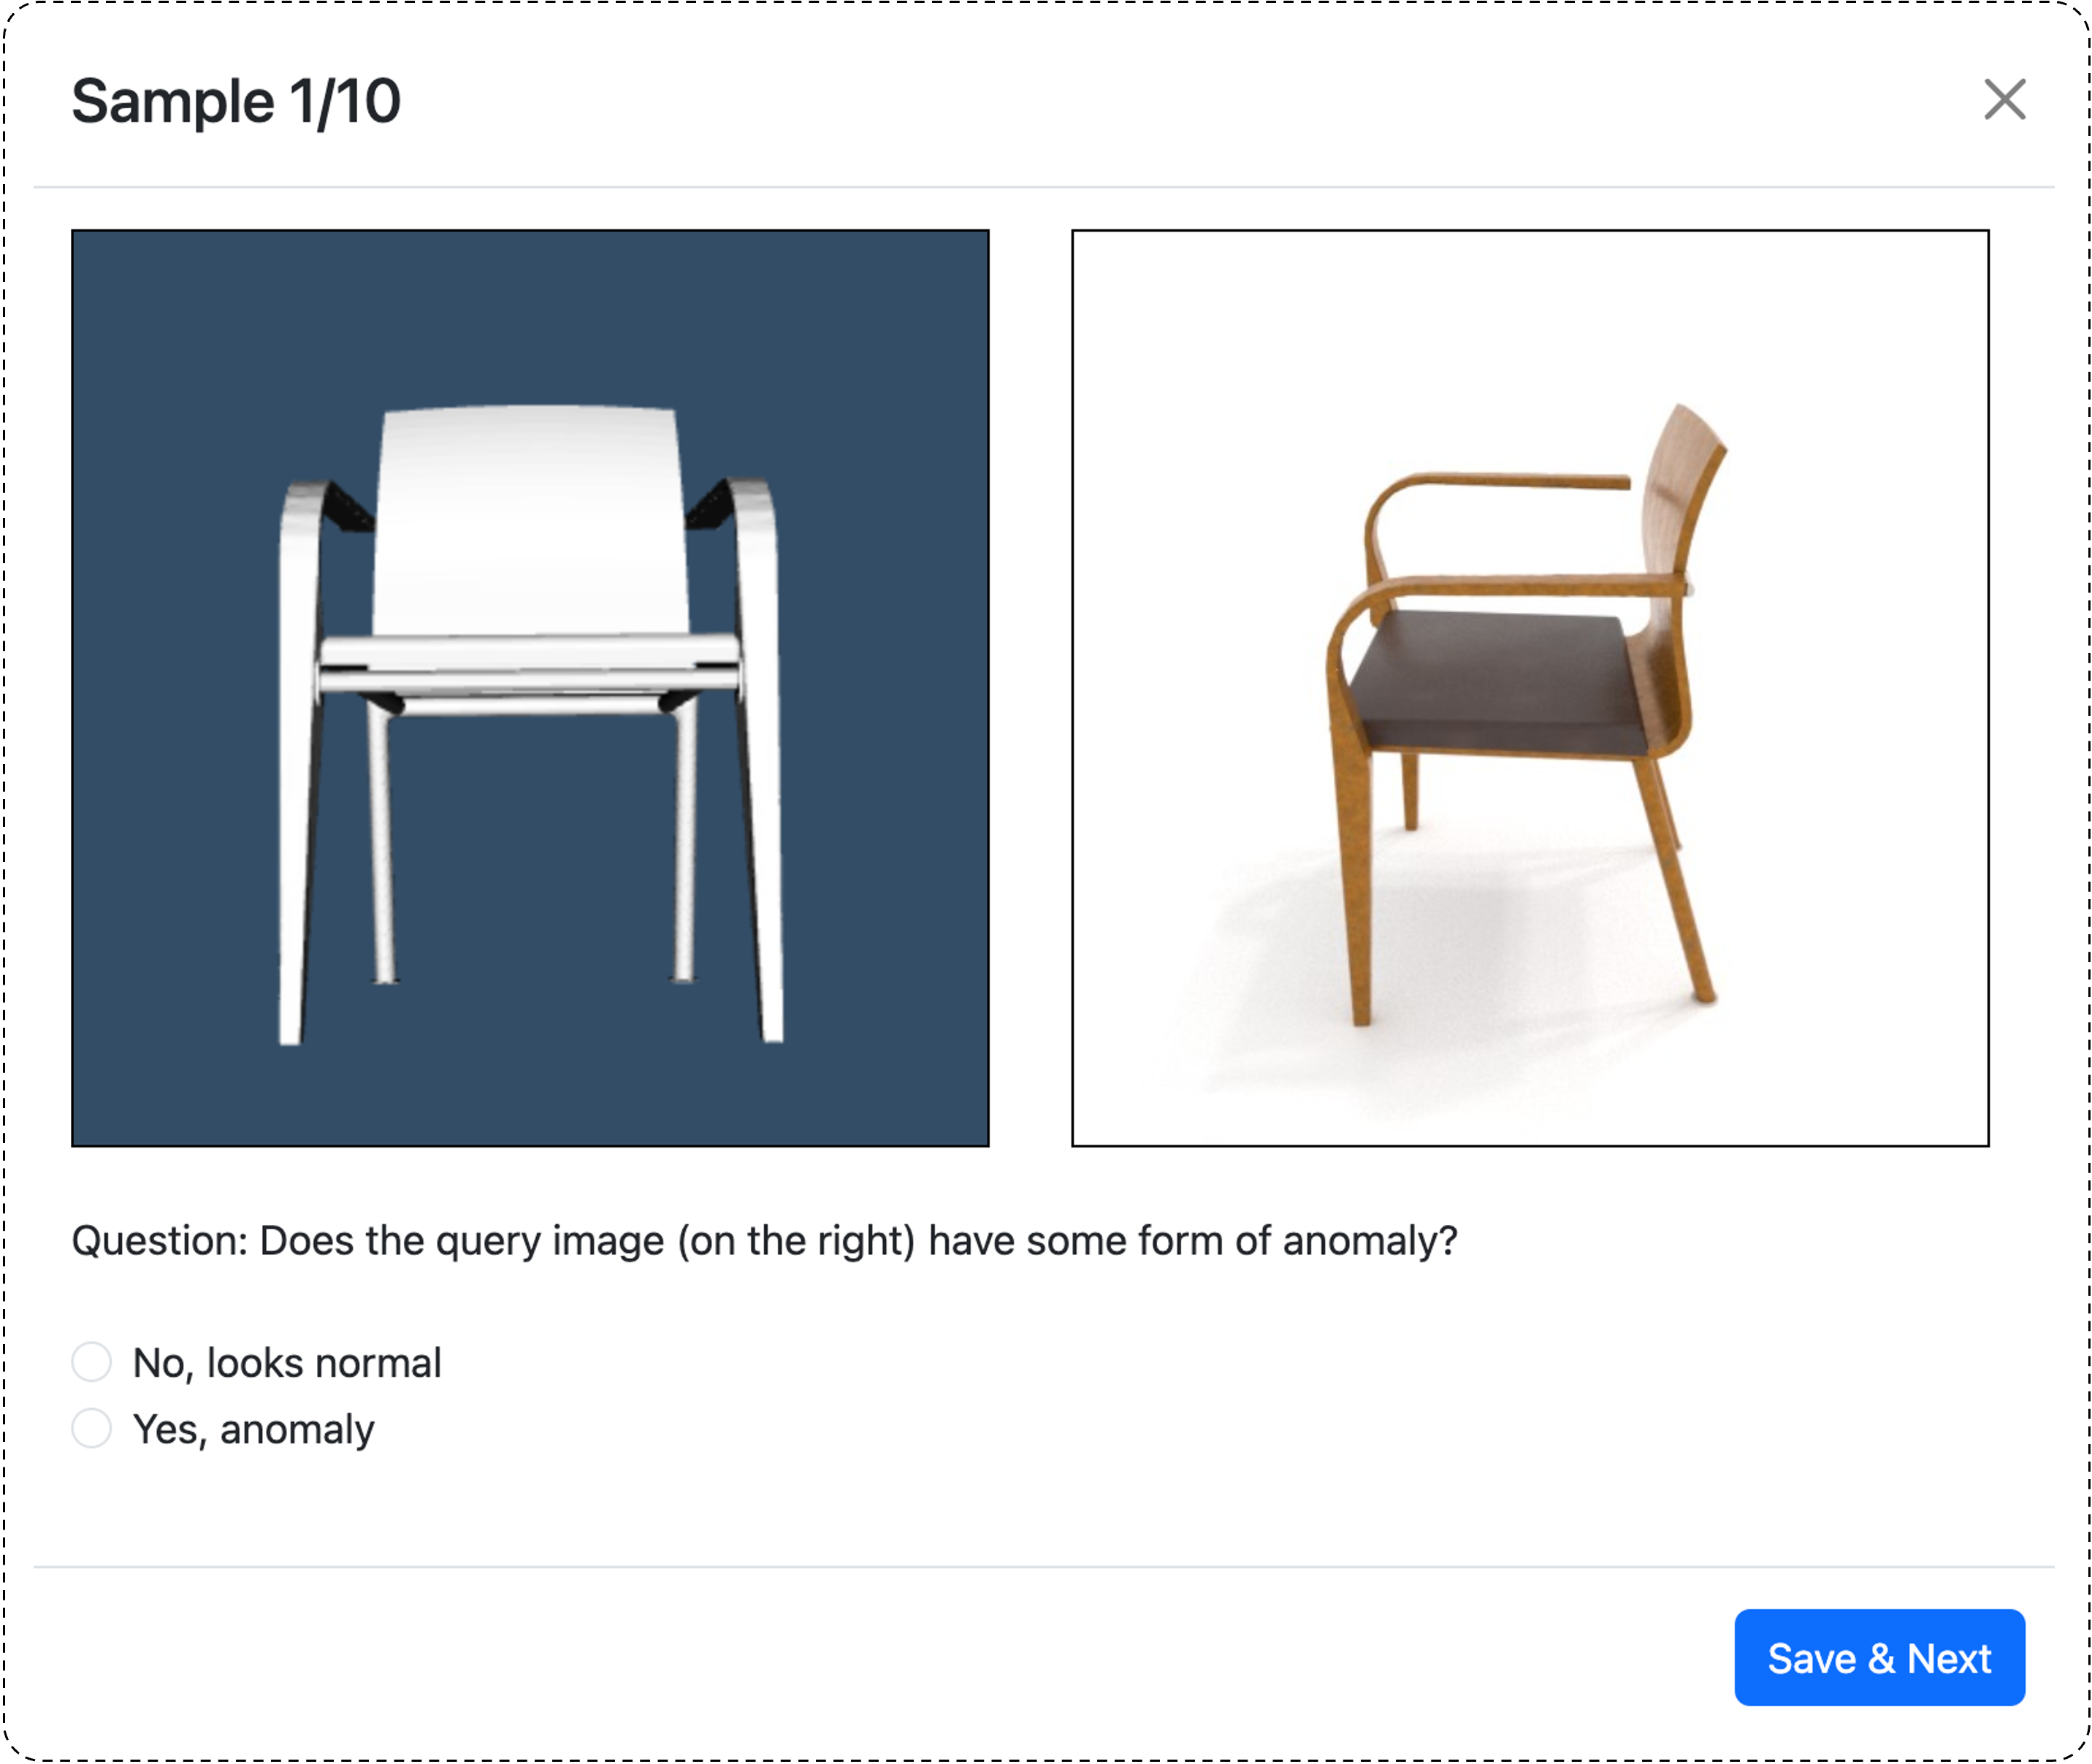}\vspace{-0.3cm}
\end{center}\vspace{-0.2cm}
\caption {Screenshot of the interface used in the user perceptual study experiment. Each participant is given a 3D model and a 2D query image of a chair and asked to check for any defects in the query image by comparing it with the 3D model. Participants can interactively explore the reference 3D model.}
\label{fig:userinterface}
 \vspace{-0.3cm}
\end{figure}

\begin{figure}[t!]
\begin{center}
   \includegraphics[width=0.99\linewidth]{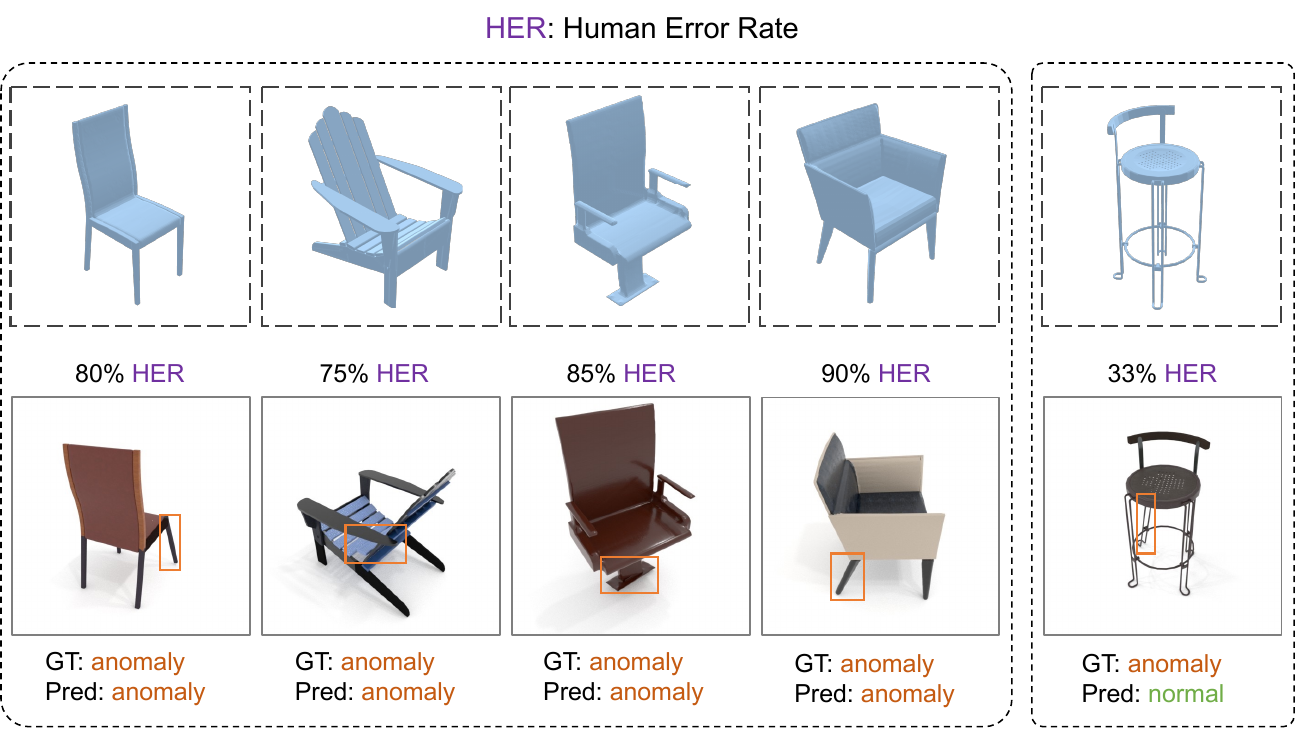}\vspace{-0.2cm}
\end{center}\vspace{-0.2cm}
\caption {\textcolor{black}{Examples illustrating cases where humans underperform (columns $1-4$) or outperform (column $5$) compared to the CMT are presented}. The Human Error Rate (HER) represents the cumulative error rate of human participants for each image. Ground truths and predictions of the CMT are displayed beneath each image. Ground truth bounding boxes are shown in orange.}
% \CJ{3D reference is needed, otherwise, it is hard to understand if anomaly is presented; which side is outperform cases?} - \AB{with the ref shape also it is bit difficult to identify the anomaly, also indicated by the poor performance by humans in the examples. }}
\label{fig:uservisual}
 \vspace{-0.3cm}
\end{figure}

\section{Qualitative Results of Anomaly Localization}
\label{sec:bbox}
Fig.~\ref{fig:bbox} illustrates the qualitative results of bounding box regression. The CMT performs better than a ViT-based model that only uses query image to make predictions.% (left column: row 3 and right column: row 1,3).  
\begin{figure*}[t!]
\begin{center}
   \includegraphics[width=1\linewidth]{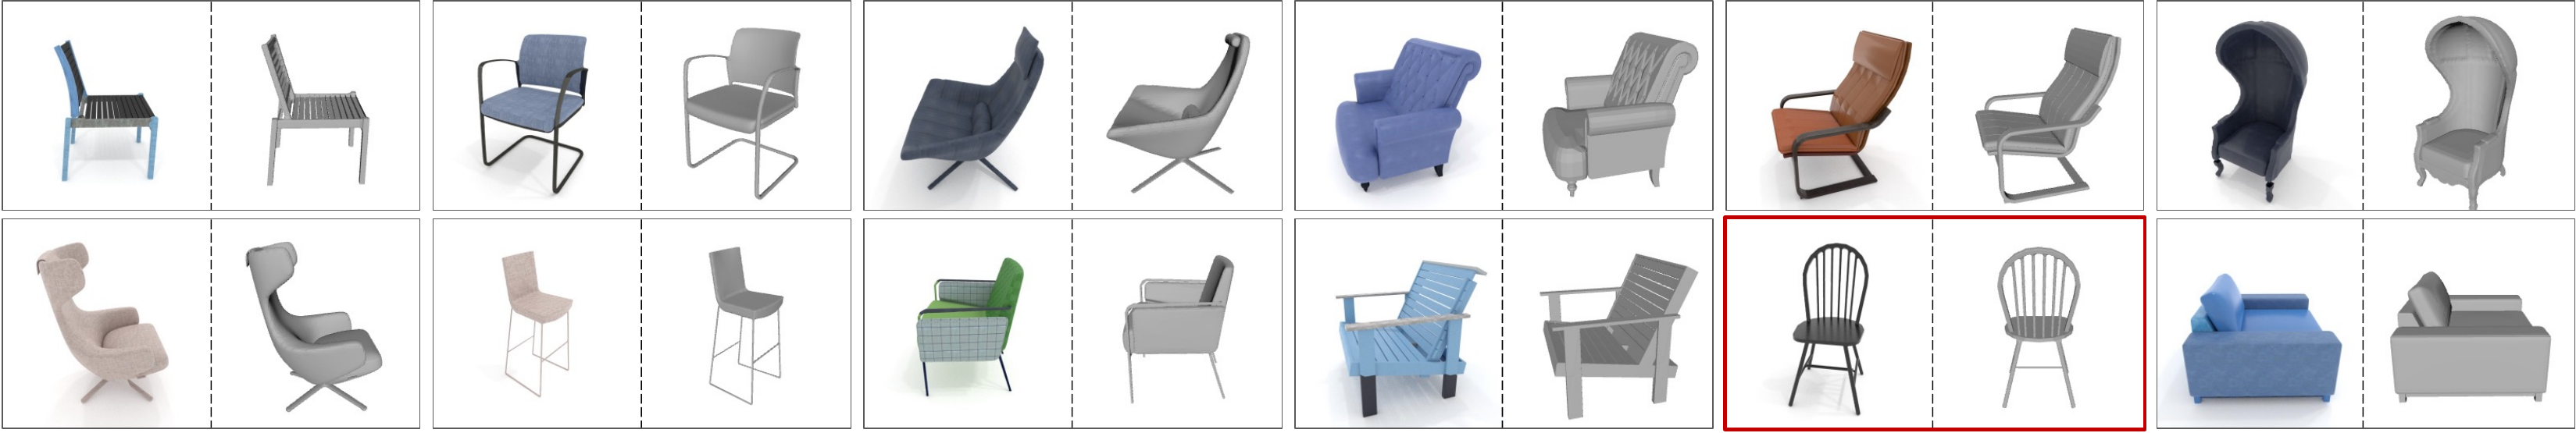}\vspace{-0.4cm}
\end{center}\vspace{-0.2cm}
\caption{Query pose estimation using learned correspondence mapping. Failure case(s) are marked in red.}
\label{fig:pose}
 \vspace{-0.2cm}
\end{figure*}

\section{Additional Details of View Prediction}
\label{sec:view}
In the view prediction experiment, we utilize 20 regularly sampled viewpoints, from which the model selects the closest viewpoint for a given query image. While the viewpoint predicted using this process will be coarse in nature, it demonstrates our model's ability to implicitly learn the relationship between the query image and the closest view. We compare our method with a ResNet model trained for 15 epochs. The ResNet model predicts the discretized pose (through classification) given only the RGB normal images as input. The training is done in a supervised setting using softmax classification loss. In contrast, our model has access to the multi-view images along with the normal RGB image, however, the training is conducted in an unsupervised way (\ie, the ground truth camera pose label was not used during training); our model learns the pose implicitly by matching the multi-view images.

Fig.~\ref{fig:pose} illustrates the qualitative results of our method showing the chair image and its matched multi-view image with the closest viewpoint.

\section{Qualitative Results on Unseen Categories}
\label{sec:unseen}

We tested our model on three very different object categories, basket, jug, and table from the $\text{3DCoMPaT++}$~\cite{slim20233dcompat} dataset where we followed the same protocol to generate anomalies, and render the multi-view and query images.
As depicted in Fig.~\ref{fig:itw}, our method successfully generalizes to these categories in spite of being trained on chairs.

\begin{figure}[t!]
\begin{center}
   \includegraphics[width=1\linewidth]{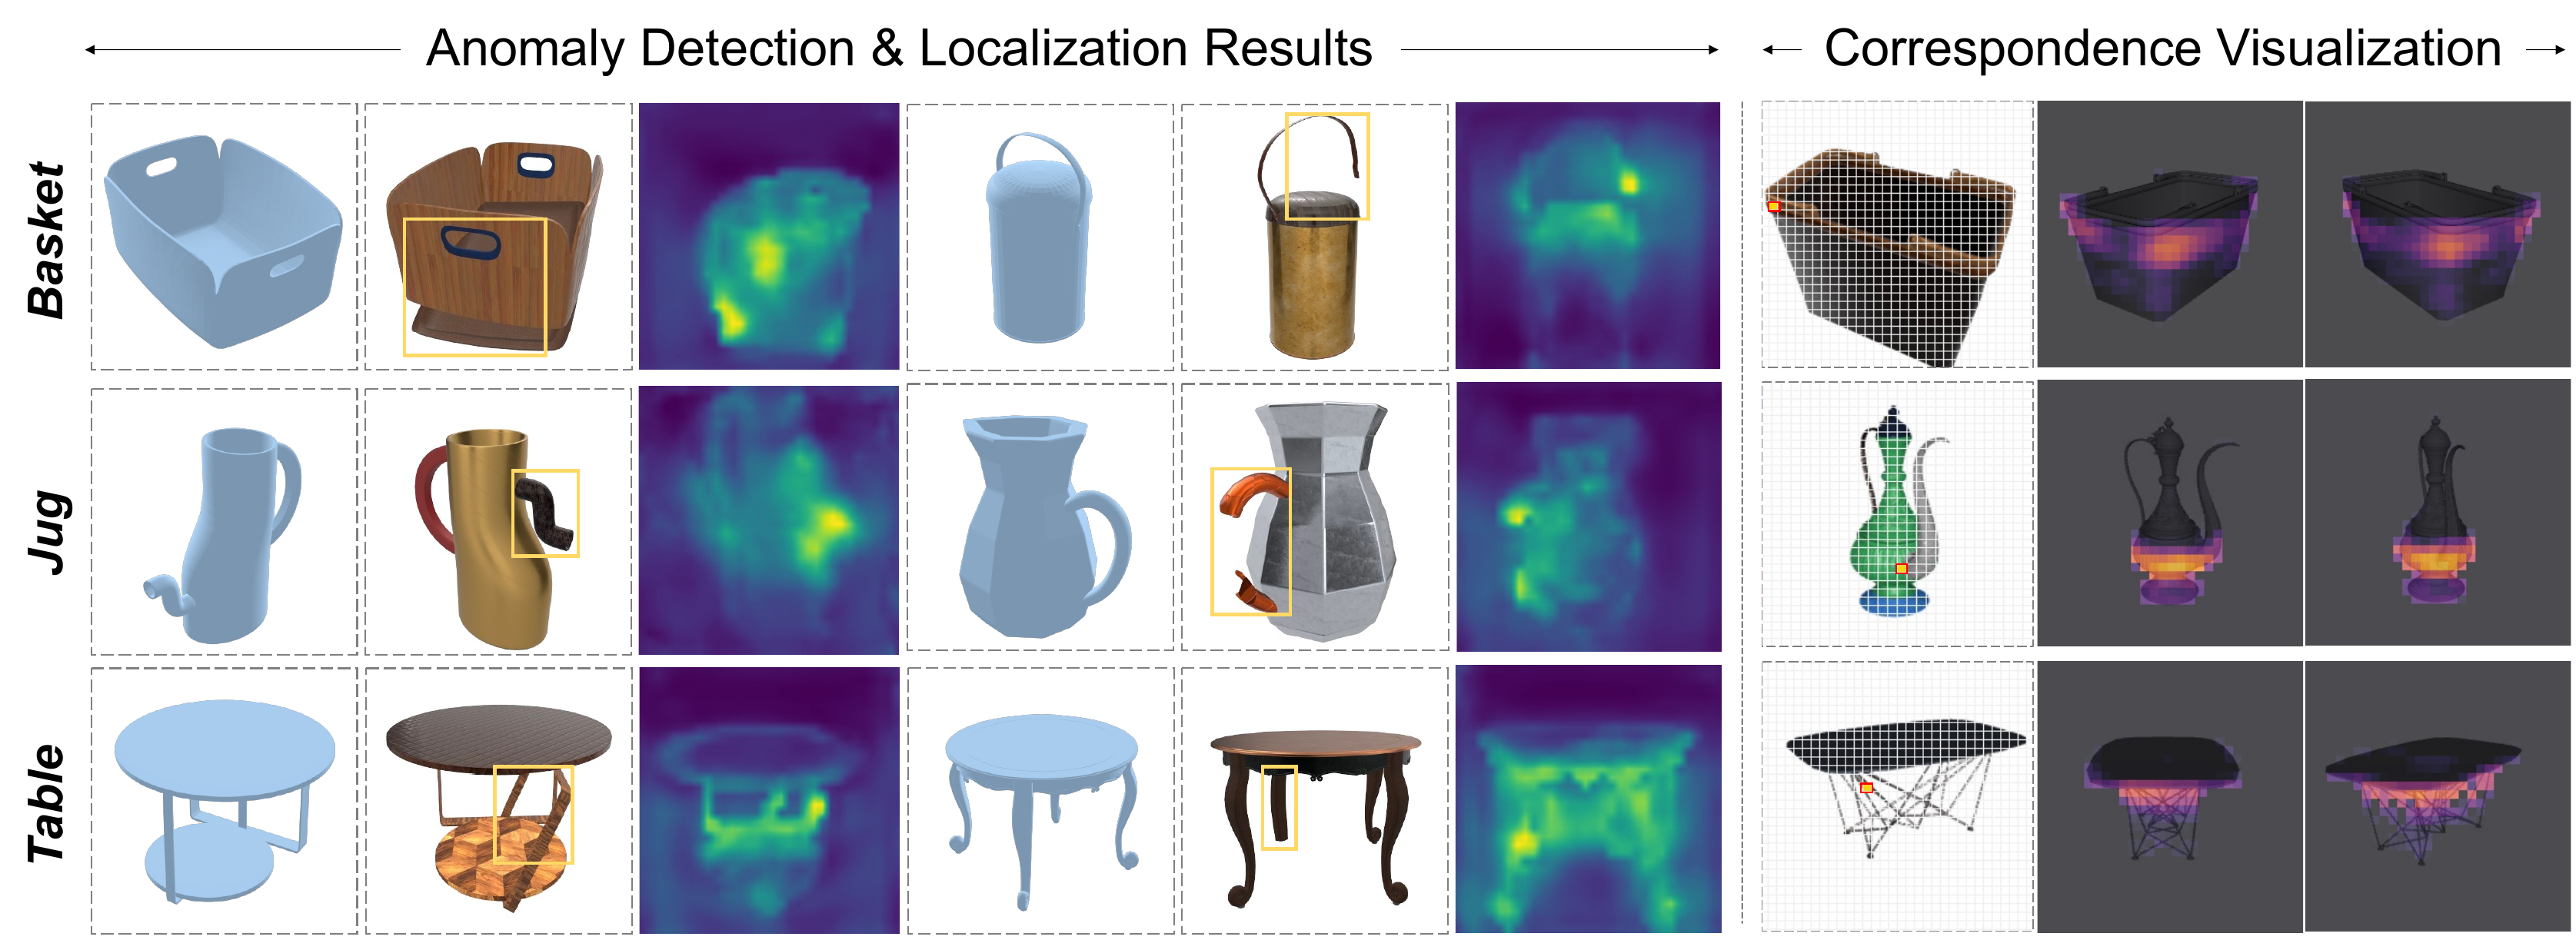}
\end{center}
\vspace{-0.6cm}
\caption{Qualitative analysis of CMT under unseen categories: (\textit{left}) For each example, we show the ref.~shape, query, and the feat.~map of the last layer of the transformer. The predicted bounding box is highlighted in yellow box. (\textit{right}) Correspondence visualization given a query patch (denoted in red square).}
\vspace{-0.4cm}
\label{fig:itw}
\end{figure}

\section{Additional Details of User Perceptual Study}
\label{sec:user}

Fig.~\ref{fig:userinterface} shows the interface used for the user perceptual study experiment. In this study, each participant is shown a reference 3D model and a query image. Then, the participants can compare the 3D model and the query side by side on the same screen and without any time restriction to give the answer. \textcolor{black}{The 3D model can be rotated freely to facilitate the comparison.} Each participant is required to provide a response to a total of 10 questions. Overall, we have collected 1000 responses from 100 participants. The outcome of the study demonstrates that our method performs better than human participants (70.6\% vs 74.8\%) on the random subset used for the study. Fig.~\ref{fig:uservisual} shows some examples where humans perform worse and better than the method. \textcolor{black}{In the first four examples, humans perform worse than the CMT. For example, in the first column, the Human Error Rate (HER) is 80\%, indicating that when the same image was presented to multiple participants, they predicted it incorrectly 80\% of the time. However, for the last example, the HER is 33\%, signifying that a higher percentage of participants correctly identified this image as an anomaly while the CMT provides a wrong prediction.}
% \CJ{Can you summarize that in specific cases, humans outperform CMT, and in some other cases, CMT is better?}
